# Supplementary material for: Video-MMLU: A Massive Multi-Discipline Lecture Understanding Benchmark
Source: arXiv:2504.14693 source file (2025-05-02)
Supplement: Supplementary file 1 [file case_study.tex]

\section{Case Study}
\label{sec:case_study}

We perform an extensive case study of~\model~on a variety of videos for video detailed captioning. As shown as followings,~\model~is capable of providing excellent detailed captions regarding the camera motion, background and main object with less hallucination. 
\begin{figure}[H]
    \centering
    \begin{tabular}{cccc}
         \subfloat{\includegraphics[width=0.22\textwidth]{fig/app_case/N13_1.pdf}} &
         \subfloat{\includegraphics[width=0.22\textwidth]{fig/app_case/N13_2.pdf}} &
         \subfloat{\includegraphics[width=0.22\textwidth]{fig/app_case/N13_3.pdf}} &
         \subfloat{\includegraphics[width=0.22\textwidth]{fig/app_case/N13_4.pdf}} \\
    \end{tabular}
    \caption{Video example of MSR-VTT~\cite{xu2016msr} benchmark.}
    \label{fig:case_study_1}
\end{figure}

\begin{figure}[H]
    \centering
    \begin{tabular}{cccc}
         \subfloat{\includegraphics[width=0.22\textwidth]{fig/app_case/N12_1.pdf}} &
         \subfloat{\includegraphics[width=0.22\textwidth]{fig/app_case/N12_2.pdf}} &
         \subfloat{\includegraphics[width=0.22\textwidth]{fig/app_case/N12_3.pdf}} &
         \subfloat{\includegraphics[width=0.22\textwidth]{fig/app_case/N12_4.pdf}} \\
    \end{tabular}
    \caption{Video example of VATEX~\cite{wang2019vatex} benchmark.}
    \label{fig:case_study_2}
\end{figure}
\begin{figure}[H]
    \centering
    \begin{tabular}{cccc}
         \subfloat{\includegraphics[width=0.22\textwidth]{fig/app_case/N14_1.pdf}} &
         \subfloat{\includegraphics[width=0.22\textwidth]{fig/app_case/N14_2.pdf}} &
         \subfloat{\includegraphics[width=0.22\textwidth]{fig/app_case/N14_3.pdf}} &
         \subfloat{\includegraphics[width=0.22\textwidth]{fig/app_case/N14_4.pdf}} \\
    \end{tabular}
    \caption{Video example.}
    \label{fig:case_study_3}
\end{figure}

\begin{figure}[H]
    \centering
    \begin{tabular}{cccc}
         \subfloat{\includegraphics[width=0.22\textwidth]{fig/app_case/N15_1.pdf}} &
         \subfloat{\includegraphics[width=0.22\textwidth]{fig/app_case/N15_2.pdf}} &
         \subfloat{\includegraphics[width=0.22\textwidth]{fig/app_case/N15_3.pdf}} &
         \subfloat{\includegraphics[width=0.22\textwidth]{fig/app_case/N15_4.pdf}} \\
    \end{tabular}
    \caption{Video example.}
    \label{fig:case_study_4}
\end{figure}

\begin{figure}[H]
    \centering
    \begin{tabular}{cccc}
         \subfloat{\includegraphics[width=0.22\textwidth]{fig/app_case/N16_1.pdf}} &
         \subfloat{\includegraphics[width=0.22\textwidth]{fig/app_case/N16_2.pdf}} &
         \subfloat{\includegraphics[width=0.22\textwidth]{fig/app_case/N16_3.pdf}} &
         \subfloat{\includegraphics[width=0.22\textwidth]{fig/app_case/N16_4.pdf}} \\
    \end{tabular}
    \caption{Video example.}
    \label{fig:case_study_5}
\end{figure}

\begin{figure}[H]
    \centering
    \begin{tabular}{cccc}
         \subfloat{\includegraphics[width=0.22\textwidth]{fig/app_case/N17_1.pdf}} &
         \subfloat{\includegraphics[width=0.22\textwidth]{fig/app_case/N17_2.pdf}} &
         \subfloat{\includegraphics[width=0.22\textwidth]{fig/app_case/N17_3.pdf}} &
         \subfloat{\includegraphics[width=0.22\textwidth]{fig/app_case/N17_4.pdf}} \\
    \end{tabular}
    \caption{Video example.}
    \label{fig:case_study_6}
\end{figure}

\begin{figure}[H]
    \centering
    \begin{tabular}{cccc}
         \subfloat{\includegraphics[width=0.22\textwidth]{fig/app_case/M21_1.pdf}} &
         \subfloat{\includegraphics[width=0.22\textwidth]{fig/app_case/M21_2.pdf}} &
         \subfloat{\includegraphics[width=0.22\textwidth]{fig/app_case/M21_3.pdf}} &
         \subfloat{\includegraphics[width=0.22\textwidth]{fig/app_case/M21_4.pdf}} \\
    \end{tabular}
    \caption{Video example.}
    \label{fig:case_study_7}
\end{figure}

\begin{figure}[H]
    \centering
    \begin{tabular}{cccc}
         \subfloat{\includegraphics[width=0.22\textwidth]{fig/app_case/M22_1.pdf}} &
         \subfloat{\includegraphics[width=0.22\textwidth]{fig/app_case/M22_2.pdf}} &
         \subfloat{\includegraphics[width=0.22\textwidth]{fig/app_case/M22_3.pdf}} &
         \subfloat{\includegraphics[width=0.22\textwidth]{fig/app_case/M22_4.pdf}} \\
    \end{tabular}
    \caption{Video example.}
    \label{fig:case_study_8}
\end{figure}

\vspace{3pt}
\begin{itemize}[leftmargin=17.5mm]
\setlength{\itemsep}{2pt}
    \item[\textbf{Example}] \textbf{Caption}
    \vspace{3pt}
    \small{
    \item[Figure~\ref{fig:case_study_1}] [short caption] A man with a mustache and a woman with a ponytail are sitting at a table.
    \item[Figure~\ref{fig:case_study_2}] [short caption] A man plays the drums in a recording studio.
    \item[Figure~\ref{fig:case_study_3}] [detailed caption] The video depicts a serene beach scene where a young woman stands on the sandy shore, gazing out towards the ocean. She is wearing a black beanie and a pink jacket, adding a pop of color to the otherwise muted scene. The beach, a vast expanse of sand, stretches out in front of her, meeting the ocean at the horizon. The ocean, a vast body of water, is visible in the background. The beach is bathed in a soft, diffused light, creating a dreamy atmosphere. The girl's gaze is directed towards the horizon, suggesting a sense of wonder or contemplation. The image is slightly blurred, adding a dreamy quality to the scene. The woman's position on the beach, coupled with the gentle waves of the ocean, suggests a moment of contemplation or admiration. The relative positions of the objects suggest a peaceful day at the beach, with the girl possibly enjoying the serene view of the ocean. The colors are mostly muted, with the girl's pink jacket standing out against the sandy beach and the blue ocean. The blurred background and the out-of-focus elements, such as the ocean and the sky, contribute to the sense of tranquility and focus on the woman. There is no text present in the video, and the colors are muted, with the exception of the pink jacket, which stands out against the more subdued tones of the surroundings.

    \item[Figure~\ref{fig:case_study_4}] [detailed caption] The video features a man with a beard and long hair, lying on the ground with his head resting on a tree trunk. He is wearing a colorful shirt with a mix of orange and green patterns. The man's face is partially obscured by the tree trunk, but his eyes are visible, looking upwards. He appears to be smiling or laughing, with his mouth open. The man's arms are crossed over his chest, suggesting a relaxed or playful posture. The background is blurred, but it appears to be a natural outdoor setting, possibly a forest or park. In the background, another person is partially visible, their presence subtly hinted at by a hand reaching out from the left side of the frame. The colors in the video are warm, with the man's shirt standing out against the muted background. The man's hair and beard are dark, and he has a light complexion. The overall mood of the video is lighthearted and carefree. There are no visible texts or other objects in the video, and the relative positions of the objects remain constant with the man in the foreground and the second person in the background. 

    \item[Figure~\ref{fig:case_study_5}] [background caption] The background features a race track with visible tire marks and barriers, surrounded by grassy areas and a few scattered trees. The track is set in a rural or semi-rural location, with hills in the distance and a cloudy sky overhead, suggesting overcast weather conditions. The track itself appears well-maintained with a smooth surface, designed for high-speed racing. The weather, indicated by the cloudy sky, contributes to the overall ambiance of the scene, enhancing the sense of a cool, possibly early morning or late afternoon setting.

    \item[Figure~\ref{fig:case_study_6}] [camera caption] The camera maintains a steady, frontal view throughout the video, capturing the woman’s expressions and the intricate details of the bookshelves. The camera starts at the right edge of the bookshelf, moving across the shelf, and ends at the left edge of the bookshelf. The framing is consistent, focusing on the woman and the bookshelves, with the camera positioned at a medium distance to the subject. This movement provides a comprehensive view of the bookshelf, showcasing the variety of books and their arrangement on the shelves. The camera occasionally pans to reveal the depth of the library, showcasing the rows of books and the inviting atmosphere. The use of natural light enhances the visual appeal, creating a warm and inviting tone throughout the video.

    \item[Figure~\ref{fig:case_study_7}] [camera caption] The view shot remains relatively static, focusing on the children playing in the backyard. The camera angle is at eye level, capturing the scene from a distance that allows both children to be visible. There is minimal camera movement, maintaining a steady focus on the children and their activities. The sequence of video frames suggests a continuous moment of play without significant changes in shooting angles or camera movement.

    \item[Figure~\ref{fig:case_study_8}] [main object caption] The main subject in the video, a black car, is seen driving down a street that appears to be in a state of disarray. The car moves steadily forward, navigating around obstacles such as a blue car parked on the side of the road. The car's movement is smooth and continuous, suggesting it is either in motion or has just come to a stop. The environment around the car is chaotic, with debris scattered across the road and signs of destruction, indicating a recent event or disaster. The car's position remains central in the frame, with the camera angle focused on it from a slightly elevated perspective, possibly from a vehicle or a structure above.

    }
\end{itemize}
