# Supplementary material for: Video-MMLU: A Massive Multi-Discipline Lecture Understanding Benchmark
Source: arXiv:2504.14693 source file (2025-05-02)
Supplement: Supplementary file 2 [file frame_caption.tex]

\section{Frame Caption Generation Prompt Template}
\label{sec:frame_caption}

Following~\cite{ju2024miradata}, we utilize LLM to generate structured detailed captions. Given an input video, LLM return five detailed captions, including camera caption, short caption, background caption, main object caption and detailed caption for the entire video guided by our designed prompt template. The complete prompt is shown as followings:

\vspace{3pt}
\begin{itemize}[leftmargin=12.5mm]
\setlength{\itemsep}{2pt}
    \item[\textbf{Type}] \textbf{Prompt}
    \vspace{3pt}
    \small{
    \item[SYSTEM] You are describing the video. Please provide detailed captions of the video from different aspects.
    \item [User] Please provide detailed and comprehensive captions for the following content:
    1. Short Caption: Summarize the video in one detailed sentence, capturing key actions and the overall mood.
    2. Background Caption: Provide a detailed description of the background, including objects, location, weather, time, and any dynamic elements such as movements in the environment.
    3. Main Object Caption: Give a thorough description of the main subject's actions, attributes, interactions, and movements throughout the video frames, including changes in posture, expression, or speed.
    4. Camera Caption: Describe the camera work in detail, including shot types, angles, movements, transitions, and any special effects used to enhance the video.
    5. Reference Caption: Generate a detailed dense caption for the video that is at least 300 words long. The caption should capture all visible actions, environmental details, and the overall emotional atmosphere in depth. Describe in detail the interactions between the main subjects and their environment, including subtle nuances of their movements or expressions. Elaborate on the sounds, textures, and other sensory experiences depicted in the video. Discuss the camera techniques used extensively, including shot types, angles, movements, and transitions. Highlight the mood and tone of the video throughout, creating a rich narrative that connects viewers emotionally to the scene. Include comprehensive descriptions of background elements that add context and depth, such as weather conditions, time of day, and cultural or historical settings. Make sure to provide a vivid portrayal that is engaging, informative, and rich enough for AI to re-generate the video content.

    No need to provide summary content. Do not describe each frame individually. Avoid using phrases like 'first frame'. The description should be rich enough for AI to re-generate the video. Please generate the response as a Python dictionary string with keys like 'short caption'. DO NOT PROVIDE ANY OTHER OUTPUT TEXT OR EXPLANATION. Only provide the Python dictionary string. 

    These are the frames from the video: [VIDEO KEYFRAME INPUT]

    \item[\texttt{GPT-4o}] Short Caption: In a sunny outdoor setting, two workers engage in a collaborative effort to prepare a gravel base for a construction project, showcasing teamwork and focus. 
    
    Camera Caption: The camera captures the scene from a low angle, providing a unique perspective that emphasizes the workers' actions and the surrounding environment. The shots are primarily medium close-ups, focusing on the workers' upper bodies and hands as they interact. The camera occasionally shifts to a wider angle, revealing more of the workspace and background elements. There are smooth transitions between shots, maintaining a steady flow that enhances the viewer's engagement with the unfolding narrative. The use of a slightly fish-eye lens effect adds depth to the scene, making the environment feel more immersive.
    Background Caption: The scene is set in a residential area with a well-maintained lawn and a brick wall partially constructed in the background. The ground is covered with a white plastic sheet, and scattered gravel is visible. A few wooden planks lie on the ground, and tools are scattered around, including a black water bottle and a power tool. 
    
    Main Object Caption: The main subjects are two workers, one wearing a gray sweatshirt and gloves, and the other dressed in casual work attire. They are actively engaged in conversation, with the first worker gesturing with his hands to emphasize points while explaining the task at hand. His posture is relaxed yet focused, indicating a collaborative atmosphere. The second worker listens attentively, occasionally nodding and responding with gestures, showcasing a dynamic interaction. Both workers exhibit a sense of camaraderie and professionalism as they prepare for the next steps in their project.
    
    Reference Caption: The video unfolds … (300 words) … through them.

    \item[User] The video has been describe from the following aspects:1. short caption: {short caption}, 2. background caption: {background caption}, 3. main object caption: {main object caption}, 4. camera caption: {camera caption}, 5.Reference Caption: {reference caption} Please generate a detailed dense caption for the video that is pretty long. You should expand the reference caption upon the information provided in the short caption, background caption, main object caption, and camera caption. Ensure that the detailed caption does not introduce any new entities or relationships that were not mentioned in the previous captions. Make sure to provide a vivid portrayal that is engaging, informative, and rich enough for AI to re-generate the video content. "Avoid using phrases like 'first frame', 'short caption', 'background caption', 'main object caption', and 'camera caption'. The description should be rich enough for AI to re-generate the video.

    \item[\texttt{GPT-4o}] Detailed Caption: The video opens with … (500 words) … literature that surrounds them.

    \item[User] [Manually check and refine]
}
\end{itemize}
