# Supplementary material for: Video-MMLU: A Massive Multi-Discipline Lecture Understanding Benchmark
Source: arXiv:2504.14693 source file (2025-05-02)
Supplement: Supplementary file 3 [file case_study.tex]

\section{Case Study}
\label{sec:case_study}
