# Supplementary material for: Video-MMLU: A Massive Multi-Discipline Lecture Understanding Benchmark
Source: arXiv:2504.14693 source file (2025-05-02)
Supplement: Supplementary file 4 [file list.tex]

1. channel的youtube链接
2. benchmark generation prompt template
3. evaluation prompt template
4. case study
8. word cloud for both caption and questions
9. calculate the failure cases percentage, the accuracy before and after filter
10.十个人的topic，平均视频长度，平均caption长度
11. 补充材料记得把视频扔进去
12. more resuts for llm
13. keyframe for each channel, table
14. caption construction pipeline
15. 补一个不同学科的text embedding图
16. different token merge ratio for auroracap的caption
17. token reduction的model的结果的table
18. token merge 的related work
19. figure 4的大大图
20.evaluation details
21. detailed caption prompts
